# Supplementary material for: Rushing Full Speed with LTE-Advanced is Economical -- A Power Consumption Analysis
Source: arXiv:1702.05251 source file (2020-02-20)
Supplement: Supplementary file 2 [file additional-CA-power-S5.tex]

\documentclass[preview]{standalone}

\providecommand{\datapath}{.}

\usepackage[utf8]{inputenc}

\usepackage{tikz}
\usepackage{pgfplots}
\pgfplotsset{compat=newest}
\usetikzlibrary{positioning, spy}
\usepackage{siunitx} %
\usepackage{sansmath}

\begin{document}

\begin{tikzpicture}[spy using outlines={circle, magnification=4, connect spies}, font=\sffamily\footnotesize]
\begin{sansmath}

\pgfplotstableread[row sep=\\,col sep=&]{
	PCC & SCC800 & SCC1800 & SCC2600 \\
	800     & 0  & 273  & 323  \\
	1800     & 300 & 190  & 310  \\
	2600    & 310 & 310 & 190 \\
}\mydataG

\pgfplotstableread[row sep=\\,col sep=&]{
	PCC & SCC800 & SCC1800 & SCC2600 \\
	800     & 300  & 339  & 403  \\
	1800     & 314 & 307  & 394  \\
	2600    & 330 & 310 & 330 \\
}\mydataS

    \begin{axis}[
	ybar,
	width= 235.0pt,			%
	height=5.5cm,
	enlarge x limits=0.3,
	ymin=0, ymax=550,
    symbolic x coords={800,1800,2600},
    bar width=0.5cm,
    xtick=data,
    nodes near coords,
	xlabel={Primary Component Carrier Frequency [\si{\mega\hertz}]},
	ylabel={Power Consumption [\si{\milli\watt}]},
	legend cell align=left,
 	legend pos=south east,
 	legend style={legend columns=-1,anchor=south east},
    ]
    \addplot[black, fill=white] table[x=PCC,y=SCC800]{\mydataS};
    \addplot[black, fill=gray] table[x=PCC,y=SCC1800]{\mydataS};
    \addplot[black, fill=black] table[x=PCC,y=SCC2600]{\mydataS};
    \legend{SCC 800, SCC 1800, SCC 2600}
        
    \end{axis}
    
	\node[draw] (label) at (3.4cm,3.6cm) {Intra-Band CA};
	\draw[-stealth] (label) -| +(-2.7cm,-1.0cm);
	\draw[-stealth] (label) -| +(2.6cm,-0.8cm);
	\draw[-stealth] (label) -- +(0cm,-1.0cm);

	\node[draw, fill=white] at (-4mm,-4mm) {DUT-B};

\end{sansmath}
\end{tikzpicture}
\end{document}
